# Supplementary material for: Simulation-to-Real domain adaptation with teacher-student learning for endoscopic instrument segmentation
Source: arXiv:2103.01593 source file (2021-03-02)
Supplement: Supplementary file 1 [file supplementary.tex]

%\textbf{\large Supplemental Material}
\section{Supplemental Material}

% Prefix a "S" to all equations, figures, tables and reset the counter
\setcounter{equation}{0}
\setcounter{figure}{0}
\setcounter{table}{0}
\setcounter{page}{1}
\setcounter{section}{0}

%\renewcommand{\bibnumfmt}[1]{[S#1]}
%\renewcommand{\citenumfont}[1]{S#1}

%\section{Supplemental Material}

\section{Hyper-parameters}

text...

\section{Implementation Details}

text...

\section{Data Perturbation Schemes}

% We use a set of perturbation policies of varying strength for training of the DNN model. The (randomly) varying strength of the policies ensures that the DNN does not end up learning the policies but useful features for segmentation.
We apply data augmentation in three forms: base, pixel intensity and pixel corruption.
Apply as weak and strong
Source contains all three but target data has without base.

\begingroup
\begin{table}[htbp] 
	\centering
	\captionsetup{justification=centering}
	\caption{List of perturbation schemes}
	\label{table:perturbation_schemes}
	\begin{tabular}{| c | c | c | c |}
    	\hline
    	Perturbation & Description & Parameter & Range \\
    	\hline
    	\hline
    	Rotate & Rotates the image (in degrees) & $\theta$ & [-30, 30] \\
	    \hline
\end{tabular}
\end{table}
\endgroup

%\bibliographystyle{IEEEtran}
%\bibliography{IEEEabrv,SupplementaryBibliography}
